# Supplementary material for: A determination of mc(mc) from HERA data using a matched heavy-flavor scheme
Source: arXiv:1605.01946 source file (2016-05-06)
Supplement: Supplementary file 1 [file appendixA.tex]

\section{Implementation of the FONLL scheme with
  $\overline{\mbox{MS}}$ masses}\label{app:implementation}

In this appendix we will describe in some detail the implementation of
the FONLL scheme in terms of the $\overline{\mbox{MS}}$ heavy-quark
running masses in {\tt APFEL}.  Starting from the more used definition
of structure functions and in terms of pole masses, our goal is to
consistently replace them with the $\overline{\mbox{MS}}$ mass
definition.

\subsection{$\overline{\mbox{MS}}$ mass vs. pole mass}

The (scale independent) pole mass $M$ and the (scale dependent)
$\overline{\mbox{MS}}$ mass $m(\mu)$ arise from two different
renormalization procedures and in perturbation theory they can be
expressed one in terms of the other. The relation connecting pole and
$\overline{\mbox{MS}}$ mass definitions has been computed in
Ref.~\cite{Chetyrkin:1999qi} up to four loops. However, in the
following we will only need to go up to one loop and thus we report
here the corresponding relation:
\begin{equation}\label{eq:PoleToMSbar}
%\frac{M}{m(\mu)} = 1 +
%h^{(1)}a_s+\underbrace{C_F\left[C_Fh_1^{(2)}+C_Ah_2^{(2)}+T_R\left(N_Lh_3^{(2)}+h_4^{(2)}\right)\right]}_{h^{(2)}}a_s^2+\mathcal{O}(a_s^3)\,,
\frac{M}{m(\mu)} = 1 + h^{(1)}a_s+\mathcal{O}(a_s^2)\,,
\end{equation}
with:
\begin{equation}\label{eq:CoeffPoleToMSbar}
\begin{array}{l}
\displaystyle h^{(1)}(\mu,m(\mu)) = C_F\left(4 + 3L_{\mu m}\right)\,,%\\
%\\
%\displaystyle h_{1}^{(2)}(\mu,m(\mu)) = -\frac{7}{8} + 30\zeta_2 + 12\zeta_3 - 48\zeta_2\ln(2) - \frac{9}2L_{\mu m} + \frac92 L_{\mu m}^2\,,\\
%\\
%\displaystyle h_{2}^{(2)}(\mu,m(\mu)) = \frac{1111}{24} - 8\zeta_2 - 6\zeta_3 + 24\zeta_2\ln(2) + \frac{185}6L_{\mu m} + \frac{11}2 L_{\mu m}^2\,,\\
%\\
%\displaystyle h_{3}^{(2)}(\mu,m(\mu)) = - \frac{71}{6} - 8\zeta_2 - \frac{26}3L_{\mu m} - 2 L_{\mu m}^2\,,\\
%\\
%\displaystyle h_{4}^{(2)}(\mu,m(\mu)) = -\frac{143}{6} + 16\zeta_2 - \frac{26}3L_{\mu m} - 2 L_{\mu m}^2\,,\\
\end{array}
\end{equation}
%where $N_L$ is the number of light (massless) quarks ($e.g.$ $N_L=3$
%for the the charm quark and $N_L=4$ for the bottom quark) and 
%$C_F=4/3$, $C_A=3$ and $T_R=1/2$ are the usual QCD color 
%factors. Moreover, we have defined:
where $C_F=4/3$ is one of the usual QCD color factors. Moreover, we
have defined:
\begin{equation}
a_s\equiv a_s(\mu) = \frac{\alpha_s(\mu)}{4\pi}\,.
\end{equation}
and:
\begin{equation}
L_{\mu m} = \ln\frac{\mu^2}{m^2(\mu)}\,.
\end{equation}
In the following we will use eq. (\ref{eq:PoleToMSbar}) to replace the
pole mass $M$ with the $\overline{\mbox{MS}}$ mass $m(\mu)$.

\subsection{RGE solution for the $\overline{\mbox{MS}}$ running mass}

In order to evaluate the running of $m(\mu)$ with the renormalization
scale $\mu$ we have to solve the corresponding renormalization-group
equation (RGE):
\begin{equation}\label{eq:massRGE}
\mu^2\frac{dm}{d\mu^2} = m(\mu)\gamma_m(a_s) = -m(\mu)\sum_{n=0}^{\infty}\gamma_m^{(n)}a_s^{n+1}\,,
\end{equation}
whose first three coefficients can be taken from
Ref.~\cite{Chetyrkin:1999pq}\footnote{The following expressions have
  been adjusted taking into account our definition of $a_s$ which
  differs by a factor of 4 with respect to that of Ref.~\cite{Chetyrkin:1999pq}.}:
\begin{subequations} 
\begin{equation}
\gamma_m^{(0)} = 4 \,,
\end{equation}
\begin{equation}
\gamma_m^{(1)} = \frac{202}3 - \frac{20}{9}N_f\,,
\end{equation}
\begin{equation}
\gamma_m^{(2)} = 1249 - \left(\frac{2216}{27}+\frac{160}{3}\zeta_3\right)N_f-\frac{140}{81}N_f^2\,,
\end{equation}
\end{subequations} 
where $N_f$ is the number of active flavours. In addition the RGE for
the running of $\alpha_s$ reads:
\begin{equation}\label{eq:alphasRGE}
\mu^2\frac{da_s}{d\mu^2} = \beta(a_s) = -\sum_{n=0}^{\infty}\beta_n a_s^{n+2}\,,
\end{equation}
with:
\begin{subequations} 
\begin{equation}
\beta_0 = 11-\frac23 N_f \,,
\end{equation}
\begin{equation}
\beta_1 = 102 - \frac{38}3 N_f\,.
\end{equation}
\begin{equation}
\beta_2 = \frac{2857}{2} - \frac{5033}{18}N_f + \frac{325}{54}N_f^2\,.
\end{equation}
\end{subequations} 
Combining eqs.~(\ref{eq:massRGE}) and~(\ref{eq:massRGE}) we obtain the
following differential equation:
\begin{equation}\label{runmass}
\frac{dm}{da_s} = \frac{\gamma_m(a_s)}{\beta(a_s)}m(a_s)\,,
\end{equation}
whose solution is:
\begin{equation}\label{eq:massRGEsolution}
m(\mu) = m(\mu_0)\exp\left[\int_{a_s(\mu_0)}^{a_s(\mu)}\frac{\gamma_m(a_s)}{\beta(a_s)}da_s\right]\,.
\end{equation}
In order to get an analytical expression out of
eq.~(\ref{eq:massRGEsolution}), we expand the integrand in the
l.h.s. using the perturbative expansions of $\gamma_m(a_s)$ and
$\beta(a_s)$ given in eqs.~(\ref{eq:massRGE})
and~(\ref{eq:alphasRGE}). This allows us to solve the integral
analytically, obtaining:
\begin{equation}\label{eq:massRGEsolutionAnal}
\begin{array}{rcl}
m(\mu)&=&\displaystyle m(\mu_0)\left(\frac{a}{a_0}\right)^{c_0}\\
\\
&\times&\displaystyle
         \frac{1+(c_1-b_1c_0)a+\frac12[c_2-c_1b_1-b_2c_0+b_1^2c_0+(c_1-b_1c_0)^2]a^2}{1+(c_1-b_1c_0)a_0+\frac12[c_2-c_1b_1-b_2c_0+b_1^2c_0+(c_1-b_1c_0)^2]a_0^2}\,,
\end{array}
\end{equation}
where we have defined:
\begin{equation}\label{eq:SolCoefs}
b_i = \frac{\beta_i}{\beta_0}\quad\mbox{and}\quad c_i = \frac{\gamma_m^{(i)}}{\beta_0}\,,
\end{equation}
and $a\equiv a_s(\mu)$ and $a_0\equiv a_s(\mu_0)$.
Eq.~(\ref{eq:massRGEsolutionAnal}) represents the
next-to-next-lo-leading order (NNLO) solution of the RGE for the
$\overline{\mbox{MS}}$ mass $m(\mu)$. 

Of course, the NLO and the LO solutions can be easily extracted from
eq.~(\ref{eq:massRGEsolutionAnal}) just by disregarding the terms
proportional to $a^2$ and $a_0^2$ for the NLO solution and also the
terms proportional to $a$ and $a_0$ for the LO solution\footnote{In
  order to be consistent, the evaluation of $a$ and $a_0$
  eq.~(\ref{eq:massRGEsolutionAnal}) must be performed at the same
  perturbative order of $m(\mu)$. So, for instance, if one wants to
  evaluate the NNLO running of $m(\mu)$ also the value of $a$ and
  $a_0$ must be computed using the NNLO running.}.

\subsection{Matching conditions}\label{sec:MatchingConditions}

When working in the context of a variable-flavour-number scheme
(VFNS), all running quantities are often required to cross the
heavy-quark thresholds to evolve from one scale to another. Such a
transition in turn requires to match in correspondence of a given
heavy-quark threshold different factorization schemes whose content of
light quarks differs by one unity. In other words, if the perturbative
evolution leads from an energy region where (by definition) there are
$N_f-1$ light flavours to another region where there are $N_f$ light
flavours, the two regions must be consistently connected and such a
connection can be perturbatively evaluated and goes under the name of
\textit{matching conditions}.

In general, the matching conditions give rise to discontinuities of
the running quantities in correspondence of the matching scale and in
the following we will report the matching conditions up to NNLO in
terms of the $\overline{\mbox{MS}}$ heavy-quark thresholds for:
$\alpha_s(\mu)$, $m(\mu)$ and PDFs.

\subsubsection*{Matching of $\alpha_s(\mu)$}

The matching condition for $\alpha_s$ were evaluated in
Ref.~\cite{Chetyrkin:1997sg} to three loops.  We report here the
relation up to two loops (again taking into account the factor 4
coming from the different definitions of $a$):
\begin{equation}\label{eq:alphaspole}
\frac{a^{(N_f-1)}(\mu)}{a^{(N_f)}(\mu)}=1-\frac23 L_{\mu M}a^{(N_f)}(\mu)+\left(\frac49L_{\mu M}^2-\frac{38}3L_{\mu M}-\frac{14}3\right)[a^{(N_f)}(\mu)]^2\,.
\end{equation}
$M$ being the pole mass of the $n$-th flavour. From
eq.~(\ref{eq:PoleToMSbar}) we can easily infer that:
\begin{equation}
\ln M^2 = \ln m^2(\mu) + 2\ln[1+h^{(1)}(\mu)a^{(N_f)}(\mu)]= \ln m^2(\mu) + 2h^{(1)}(\mu)a^{(N_f)}(\mu)+\mathcal{O}([a^{(N_f)}]^2)\,.
\end{equation}
Therefore it is straightforward to see that:
\begin{equation}\label{eq:conversionLog}
L_{\mu M}  = L_{\mu m} - 2h^{(1)}a^{(N_f)}=L_{\mu m}-\left(\frac{32}3+8L_{\mu m}\right)a^{(N_f)}\,,
\end{equation}
so that:
\begin{equation}\label{eq:alphasmsbar}
\frac{a^{(N_f-1)}(\mu)}{a^{(N_f)}(\mu)}=1-\frac23 L_{\mu m}a^{(N_f)}(\mu)+\left(\frac49L_{\mu m}^2-\frac{22}3L_{\mu m}+\frac{22}9\right)[a^{(N_f)}(\mu)]^2\,.
\end{equation}

In order to simplify the expression, it is a common procedure to
perform the matching in the point where the logarithms vanish. In this
particular case, choosing $\mu=m(\mu)=m(m)$, we get:
\begin{equation}
a^{(N_f-1)}(m)=a^{(N_f)}(m)\left(1+\frac{22}9[a^{(N_f)}(m)]^2\right)\,,
\end{equation}
which can be easily inverted obtaining:
\begin{equation}\label{eq:alphasatthrs}
a^{(N_f)}(m)=a^{(N_f-1)}(m)\left(1-\frac{22}9[a^{(N_f-1)}(m)]^2\right)\,.
\end{equation}

It is interesting to observe that, in order to perform the matching as
described above, one just needs to know the value of $m(m)$. This is
the so-called RG-invariant $\overline{\mbox{MS}}$ mass. This finally
allows us to evaluate the values of $a$ and $a_0$ that enter in
eq. (\ref{eq:massRGEsolutionAnal}) needed to compute the running of
$m(\mu)$.

\subsubsection*{Matching of $m(\mu)$}

Also the running of $\overline{\mbox{MS}}$ needs to be matched at the
heavy-quark thresholds. In particular, one needs to match the
$(N_f-1)$ with $(N_f)$ scheme for the mass $m_q(\mu)$, with $q=c,b,t$,
at the threshold $m_h(\mu)$, with again $h=c,b,t$ the $n$-th
threshold. From Ref.~\cite{Chetyrkin:2000yt} we read:
\begin{equation}\label{eq:mqmc}
\frac{m_q^{(N_f-1)}(\mu)}{m_q^{(N_f)}(\mu)}=1+\left(\frac43L_{\mu m}^{(h)2}-\frac{20}9L_{\mu m}^{(h)}+\frac{89}{27}\right)[a^{(N_f)}(\mu)]^2\,,
\end{equation}
where:
\begin{equation}
L_{\mu m}^{(h)} =\ln\frac{\mu^2}{m_h^2(\mu)}\,.
\end{equation}
Exactly as before, if we choose to match the two schemes at the scale $\mu=m_h(\mu)=m_h(m_h)$, the logarithmic terms vanish and we are left with:
\begin{equation}
m_q^{(N_f-1)}(m_h)=\left(1+\frac{89}{27}[a^{(N_f)}(m_h)]^2\right)m_q^{(N_f)}(m_h)\,,
\end{equation}
whose inverse is:
\begin{equation}
m_q^{(N_f)}(m_h)=\left(1-\frac{89}{27}[a^{(N_f-1)}(m_h)]^2\right)m_q^{(N_f-1)}(m_h)\,.
\end{equation}

\subsubsection*{Matching of PDFs}

To conclude the section on matching conditions, we finally consider
PDFs. One can write the singlet and the gluon in the $N_f$ scheme in
terms of singlet and gluon in the $N_f-1$ scheme at any scale $\mu$ in
the pole-mass scheme as follows:
\begin{equation}\label{eq:MatchPDFsPole}
\begin{array}{c}
\displaystyle {\Sigma^{(N_f)} \choose g^{(N_f)}}=\begin{pmatrix}1+a_s^2[A_{qq,h}^{N\!S,(2)}+\tilde{A}^{S,(2)}_{hq}] & a_s\tilde{A}^{S,(1)}_{hg}+a_s^2\tilde{A}^{S,(2)}_{hg}\\
a_s^2A^{S,(2)}_{gq,h} & 1+a_sA_{gg,h}^{S,(1)}+a_s^2A_{gg,h}^{S,(2)}\end{pmatrix}{\Sigma^{(N_f-1)} \choose g^{(N_f-1)}}\,,
\end{array}
\end{equation}
where the form of the functions entering the transformation matrix
above are given in Appendix B of Ref.~\cite{Buza:1996wv}.  We omit the
matching conditions for the non-singlet PDF combinations because there
is no $\mathcal{O}(a_s)$ correction and the first correction appears
at $\mathcal{O}(a_s^2)$. This makes the conversion from the pole to
the $\overline{\mbox{MS}}$ mass scheme ineffective up to NNLO

In order to replace the pole mass $M$ with the $\overline{\mbox{MS}}$
mass $m(\mu)$, we just have to plug eq.~(\ref{eq:conversionLog}) into
eq.~(\ref{eq:MatchPDFsPole}). In doing so, only the $\mathcal{O}(a_s)$
terms proportional to $\ln(\mu^2/M^2)$ play a role in the conversion
up to NNLO. Since the functions $\tilde{A}^{S,(1)}_{hg}$ and
$A_{gg,h}^{S,(1)}$ can be written as:
\begin{equation}\label{eq:OasMatchPDFs}
\begin{array}{l}
\displaystyle \tilde{A}^{S,(1)}_{hg}\left(x,\frac{\mu^2}{M^2}\right) = f_1(x)\ln\frac{\mu^2}{M^2}\,,\\
\\
\displaystyle A^{S,(1)}_{gg,h}\left(x,\frac{\mu^2}{M^2}\right) = f_2(x)\ln\frac{\mu^2}{M^2}
\end{array}\,,
\end{equation}
where:
\begin{equation}\label{eq:OasPDFsMatchCoeff}
\begin{array}{l}
\displaystyle f_1(x)= 4 T_R[x^2+(1-x)^2]\,,\\
\\
\displaystyle f_2(x)= -\frac43 T_R \delta(1-x)\,.
\end{array}
\end{equation}
Replacing $M$ with $m$ in eq.~(\ref{eq:OasMatchPDFs}) using
eq. (\ref{eq:conversionLog}), we get:
\begin{equation}
\begin{array}{l}
\displaystyle \tilde{A}^{S,(1)}_{hg}\left(x,\frac{\mu^2}{m^2}\right) = f_1(x)\ln\frac{\mu^2}{m^2}-2h^{(1)}(\mu)f_1(x)a_s(\mu)\\
\\
\displaystyle A^{S,(1)}_{gg,h}\left(x,\frac{\mu^2}{m^2}\right) = f_2(x)\ln\frac{\mu^2}{m^2}-2h^{(1)}(\mu)f_2(x)a_s(\mu)
\end{array}\,.
\end{equation}
Therefore eq. (\ref{eq:MatchPDFsPole}) in terms of $m$ becomes:
\begin{equation}
\begin{array}{c}
\displaystyle {\Sigma^{(N_f)}\choose g^{(N_f)}}=\begin{pmatrix}1+a_s^2[A_{qq,h}^{N\!S,(2)}+\tilde{A}^{S,(2)}_{hq}] & a_s\tilde{A}^{S,(1)}_{hg}+a_s^2[\tilde{A}^{S,(2)}_{hg}-2h^{(1)}f_1]\,,\\
a_s^2A^{S,(2)}_{gq,h} & 1+a_sA_{gg,h}^{S,(1)}+a_s^2[A_{gg,h}^{S,(2)}-2h^{(1)}f_2]\end{pmatrix}{\Sigma^{(N_f-1)} \choose g^{(N_f-1)}}\,.
\end{array}
\end{equation}

As usual, we choose to match the $N_f$ scheme to the $N_f-1$ scheme at
$\mu = m(\mu) = m(m)$ so that all the logarithmic terms vanish,
obtaining:
\begin{equation}
\begin{array}{c}
\displaystyle {\Sigma^{(N_f)}\choose g^{(N_f)}}=\begin{pmatrix}1+a_s^2[A_{qq,h}^{N\!S,(2)}+\tilde{A}^{S,(2)}_{hq}] & a_s^2[\tilde{A}^{S,(2)}_{hg}-2h^{(1)}f_1]\\
a_s^2A^{S,(2)}_{gq,h} & 1+a_s^2[A_{gg,h}^{S,(2)}-2h^{(1)}f_2]\end{pmatrix}{\Sigma^{(N_f-1)} \choose g^{(N_f-1)}}\,.
\end{array}
\end{equation}

\subsubsection*{Renormalization scale variation}

The scale $\mu$ that appears in $a_s$ and $m_q$ is the
\textit{renormalization} scale, which in this section we will indicate
with $\mu_R$.  On the other hand, the scale that explicitly appears in
the PDFs is the \textit{factorization} scale, which we will now denote
with $\mu_F$. In principle, renormalization and factorization scales
are different but in general one can write $\mu_R = \kappa \mu_F$,
where $\kappa$ can be any real number\footnote{It should be noticed
  that in the case $\kappa\neq1$ PDFs aquire an implicit dependence on
  $\mu_R$ that comes from a redefinition of the splitting functions
  that in turn derives from the expansion of $\alpha_s(\mu_R)$ around
  $\mu_R=\mu_F$ that appears in the DGLAP equation.}.

The most common choice when matching the $N_f-1$ scheme with the $N_f$
scheme is to set $\mu_F$ equal to heavy quark thresholds ($M_c$, $M_b$
and $M_t$ in the pole-mass scheme and $m_c(m_c)$, $m_b(m_b)$ and
$m_t(m_t)$ in the $\overline{\mbox{MS}}$ scheme). In doing this the
logarithmic terms in the PDF matching conditions are assured to
vanish.  On the other hand, if $\kappa$ is different from one, the
logarithmic terms in the matching conditions for $a_s(\mu_R)$ and
$m_q(\mu_R)$ do not vanish anymore. This is exactly the case when
renormalization scale variations are considered and in the
following we will show how matching condition
for $a_s$ and $m_q$ change for $\kappa\neq1$.

Let us start with $\alpha_s$. Inverting eq.~(\ref{eq:alphasmsbar}) we
obtain:
\begin{equation}
\frac{a^{(N_f)}(\mu_R)}{a^{(N_f-1)}(\mu_R)} = 1 + c_1a^{(N_f-1)}(\mu_R) + c_2 [a^{(N_f-1)}(\mu_R)]^2\,,
\end{equation}
where:
\begin{equation}
c_1 = \frac23 L_{\mu m}
\quad\mbox{and}\quad
c_2 = \frac49L_{\mu m}^2+\frac{22}3L_{\mu m}-\frac{22}9\,.
\end{equation}
Setting $\mu_F=\kappa \mu_F$ we have that:
\begin{equation}
L_{\mu m} = \ln\frac{\mu_R}{m(\mu_R)}=\ln\frac{\kappa\mu_F}{m(\kappa \mu_F)}\,.
\end{equation}
As usual, the matching scale is chosen to be $\mu_F = m(m)$, so that:
\begin{equation}
L_{\mu m} \rightarrow \ln\kappa + \ln\frac{m(m)}{m(\kappa m)}\,.
\end{equation}
But using eq.~(\ref{eq:massRGEsolution}), it easy to see that:
\begin{equation}
 \ln\frac{m(m)}{m(\kappa m)}=a_s(\kappa m)\gamma_m^{(0)}\ln\kappa+\mathcal{O}[a_s^2(\kappa m)]\,,
\end{equation}
so that:
\begin{equation}\label{eq:LmumExp}
L_{\mu m} \rightarrow [1+\gamma_m^{(0)}a_s(\kappa m)]\ln\kappa\,.
\end{equation}
It should be noticed that in the eq.~(\ref{eq:LmumExp}), since
$a_s^{(N_f-1)}=a_s^{(N_f)}+\mathcal{O}([a_s^{(N_f)}]^2)$, it does not
matter whether one puts $a_s^{(N_f)}(\kappa m)$ or
$a_s^{(N_f-1)}(\kappa m)$ because the difference would be subleading.

Therefore, setting $\mu=\mu_R=\kappa m(m) = \kappa m$ in
eq.~(\ref{eq:alphasmsbar}) and using eq. (\ref{eq:LmumExp}), one gets:
\begin{equation}
\begin{array}{rcl}
a^{(N_f-1)}(\kappa m)&=&\displaystyle a^{(N_f)}(\kappa m)\bigg\{1-\frac23
  \ln\kappa\,a^{(N_f)}(\kappa
  m)\\
\\
&+&\displaystyle \left[\frac49\ln^2\kappa-\frac{2}3\left(\gamma_m^{(0)}+11\right)\ln\kappa+\frac{22}9\right][a^{(N_f)}(\kappa
  m)]^2\bigg\}\,,
\end{array}
\end{equation}
whose inverse is:
\begin{equation}
\begin{array}{rcl}
a^{(N_f)}(\kappa m)&=&\displaystyle a^{(N_f-1)}(\kappa m)\bigg\{1+\frac23
  \ln\kappa\,a^{(N_f-1)}(\kappa
  m)\\
\\
&+&\displaystyle \left[\frac49\ln^2\kappa+\frac{2}3\left(\gamma_m^{(0)}+11\right)\ln\kappa-\frac{22}9\right][a^{(N_f-1)}(\kappa
  m)]^2\bigg\}\,.
\end{array}
\end{equation}

Now let us turn to $m_q$. In this case there is not much to do. In
fact, for an arbitary matching point the matching condition of the
$\overline{\mbox{MS}}$ mass starts at $\mathcal{O}(\alpha_s^2)$
(cfr. eq. (\ref{eq:mqmc})), threfore writing $L_{\mu m}$ in terms of
$\ln\kappa$ would give rise to subleading terms (see
eq. (\ref{eq:LmumExp})). As a consequence, up to NNLO, we have that:
\begin{equation}
m_q^{(N_f-1)}(\kappa m_h)=\left[1+\left(\frac43\ln^2\kappa-\frac{20}9\ln\kappa+\frac{89}{27}\right)[a^{(N_f)}(\kappa m_h)]^2\right]m_q^{(N_f)}(\kappa m_h)\,,
\end{equation}
and its inverse is:
\begin{equation}
m_q^{(N_f)}(\kappa
m_h)=\left[1-\left(\frac43\ln^2\kappa-\frac{20}9\ln\kappa+\frac{89}{27}\right)[a^{(N_f-1)}(\kappa
  m_h)]^2\right]m_q^{(N_f-1)}(\kappa m_h)\,.
\end{equation}

\subsection{Structure functions}

We finally turn to discuss how the $\overline{\mbox{MS}}$ masses
change the DIS massive structure functions. We will first consider the
neutral-current (NC) massive structure functions up to
$\mathcal{O}(\alpha_s^2)$, which is the highest perturbative order at
which corrections are known exactly, and then we will consider the
charged-current (CC) massive structure functions again up to the
highest perturbative order exactly known, that is
$\mathcal{O}(\alpha_s)$. In order to shorten the notation, in the
following we will adopt the following defintions:
\begin{equation}
M =\;\mbox{pole mass},\quad m\equiv m(\mu) =\;\overline{\mbox{MS}}\mbox{ mass},\quad a_s\equiv a_s(\mu),\quad h^{(l)}\equiv h^{(l)}(\mu,m(\mu))\,.
\end{equation}

\subsubsection{Neutral current}

Dropping all the unnecessary dependences, the NC massive structure
functions up to $\mathcal{O}(a_s^2)$ have the form:
\begin{equation}
F(M) = a_sF^{(0)}(M) + a_s^2F^{(1)}(M) + \mathcal{O}(a_s^3)\,.
\end{equation}
The goal is to replace explicitly the pole mass $M$ with the
$\overline{\mbox{MS}}$ mass $m$ using eq.~(\ref{eq:PoleToMSbar}). To
this end, we expand $F^{(0)}(M)$ and $F^{(1)}(M)$ around $M=m$:
\begin{equation}
F^{(l)}(M) = \sum_{n=0}^{\infty}\frac1{n!}\frac{d^n F^{(l)}}{dM^n}\bigg|_{M=m}(M-m)^n\,,
\end{equation}
so that, up to $\mathcal{O}(a_s^2)$, what we need is:
\begin{equation}
\begin{array}{l}
\displaystyle F^{(0)}(m) = F^{(0)}(m) + a_smh^{(1)}\frac{dF^{(0)}}{dM}\bigg|_{M=m}\,,\\
\\
\displaystyle F^{(1)}(M) = F^{(1)}(m)\,.
\end{array}
\end{equation}
Finally, we have that:
\begin{equation}\label{eq:changescheme}
F(m) = a_sF^{(0)}(m) + a_s^2\left[F^{(1)}(m)+mh^{(1)}\frac{dF^{(0)}}{dM}\bigg|_{M=m}\right]\,.
\end{equation}

We now need to evaluate explicitly the derivative in
eq. (\ref{eq:changescheme}). First of all we observe that:
\begin{equation}\label{eq:convolution0}
F^{(0)}(M) = x\int_x^{x_{\mbox{\tiny max}}(M)} \frac{dz}{z}g\left(\frac{x}{z}\right)C_g^{(0)}(\eta(z,M),\xi(M),\chi(M))\,,
\end{equation}
being $g$ the gluon distribution function and where we have used the
following definitions:
\begin{equation}
x_{\mbox{\tiny max}}(M)=\frac1{1+\frac{4M^2}{Q^2}},\quad\eta(z,M) = \frac{Q^2}{4M^2}\left(\frac1z-1\right)-1,\quad \xi(M) =\frac{Q^2}{M^2},\quad \chi(M) =\frac{\mu^2}{M^2}\,.
\end{equation}
Defining:
\begin{equation}
G(z,M)=\frac{x}{z}g\left(\frac{x}{z}\right)C_g^{(0)}(\eta(z,M),\xi(M),\chi(M))\,,
\end{equation}
the derivative of eq.~(\ref{eq:convolution0}) can be written as:
\begin{equation}
\frac{dF^{(0)}}{dM} = \frac{d}{dM}\int_x^{x_{\mbox{\tiny max}}(M)} dzG(z,M) = \frac{d\widetilde{G}(x_{\mbox{\tiny max}}(M),M)}{dM}-\frac{d\widetilde{G}(x,M)}{dM}\,,
\end{equation}
where $\widetilde{G}(z,M)$ is the primitive of $G(z,M)$ with respect of $z$ (i.e. $\partial\widetilde{G}/\partial z = G$). But:
\begin{equation}
\frac{d\widetilde{G}(x_{\mbox{\tiny max}}(M),M)}{dM} = \frac{d \widetilde{G}(x_{\mbox{\tiny max}},M)}{d M}+\frac{dx_{\mbox{\tiny max}}}{dM}G(x_{\mbox{\tiny max}},M)\,,
\end{equation}
thus:
\begin{equation}\label{eq:withbound}
\begin{array}{c}
\displaystyle \frac{dF^{(0)}}{dM} = \frac{\partial \widetilde{G}(x_{\mbox{\tiny max}},M)}{\partial M}-\frac{\partial\widetilde{G}(x,M)}{\partial M}+\frac{dx_{\mbox{\tiny max}}}{dM}G(x_{\mbox{\tiny max}},M) =\\
\\
\displaystyle \int_x^{x_{\mbox{\tiny max}}(M)} dz\frac{\partial G(z,M)}{\partial M}+\frac{dx_{\mbox{\tiny max}}}{dM}G(x_{\mbox{\tiny max}},M)\,.
\end{array}
\end{equation}
It can be shown that bounduary term in eq.~(\ref{eq:withbound})
vanishes ($e.g.$ see Ref.~\cite{Alekhin:2010sv}), thus it can be
omitted.

Gathering all pieces, since:
\begin{equation}
\frac{\partial G(z,M)}{\partial M} = \frac{x}{z}g\left(\frac{x}{z}\right)\frac{\partial C_g^{(0)}}{\partial M}\,,
\end{equation}
we have that:
\begin{equation}\label{eq:withoutbound}
\begin{array}{rcl}
\displaystyle \frac{dF^{(0)}}{dM}\bigg|_{M=m}&=&\displaystyle
                                                 \left[x\int_x^{x_{\mbox{\tiny
                                                 max}}(M)}\frac{dz}{z}g\left(\frac{x}{z}\right)\frac{\partial
                                                 C_g^{(0)}}{\partial
                                                 M}\right]\Bigg|_{M=m}\\
\\
&=&\displaystyle x\int_x^{x_{\mbox{\tiny
    max}}(m)}\frac{dz}{z}g\left(\frac{x}{z}\right)\left[\frac{\partial
    C_g^{(0)}}{\partial M}\right]\Bigg|_{M=m}\,.
\end{array}
\end{equation}

Finally, taking into account that:
\begin{equation}
F^{(1)}(M) = \sum_{i=q,\overline{q},g}x\int_x^{x_{\mbox{\tiny max}}(M)} \frac{dz}{z}q_i\left(\frac{x}{z}\right)C_i^{(1)}(z,M)
\end{equation}
and using eqs.~(\ref{eq:changescheme}) and~(\ref{eq:withoutbound}),
one can explicitly write down the full structure of the NNLO massive
structure functions ($F_2$ and $F_L$) in terms of $\overline{\mbox{MS}}$ masses as
follows:
\begin{equation}\label{eq:masterNC}
\begin{array}{c}
\displaystyle F(m) = x\int_x^{x_{\mbox{\tiny max}}(m)} \frac{dz}{z}g\left(\frac{x}{z}\right)\left[a_sC_g^{(0)}(z,m)+a_s^2\left(C_g^{(1)}(z,m)+mh^{(1)}\left[\frac{\partial C_g^{(0)}}{\partial M}\right]\Bigg|_{M=m}\right)\right]+\\
\\
\displaystyle \sum_{i=q,\overline{q}}x\int_x^{x_{\mbox{\tiny max}}(M)} \frac{dz}{z}q_i\left(\frac{x}{z}\right)a_s^2C_i^{(1)}(z,M)\,.
\end{array}
\end{equation}

In order to carry out the implementation, we need to evaluate
explicitly the derivative of $C_g^{(0)}$ in eq. (\ref{eq:masterNC})
and this must be done separately for $F_2$ and $F_L$.

We consider first $F_2$. The general structure of $C_{2,g}^{(0)}$ is
the following:
\begin{equation}
\begin{array}{rl}
\displaystyle C_{2,g}^{(0)}(z,Q^2,M^2)=&\displaystyle T_R\Big\{2(1-6\epsilon-4\epsilon^2)I_2(\epsilon,z)-2(1-2\epsilon)I_1(\epsilon,z)+I_0(\epsilon,z)+\\
\\
& \displaystyle -4(2-\epsilon)J_2(\epsilon,z)+4(2-\epsilon)J_1(\epsilon,z)-J_0(\epsilon,z)\Big\}\,,
\end{array}
\end{equation}
where:
\begin{equation}\label{eq:iq}
I_q(\epsilon,z) = z^q\ln\left(\frac{1+v}{1-v}\right)\,.
\end{equation}
\begin{equation}\label{eq:jq}
J_q(\epsilon,x) = z^q v\,,
\end{equation}
with:
\begin{equation}\label{eq:definitions1}
\epsilon = \frac{M^2}{Q^2}\,,\quad
a=\frac1{1+4\epsilon}\quad\mbox{and}\quad v=\sqrt{1-4\epsilon\frac{z}{1-z}}\,.
\end{equation}
From the definitions in eq.~(\ref{eq:definitions1}), we obtain:
\begin{equation}\label{eq:derivatives}
\begin{array}{rl}
\displaystyle \frac{\partial}{\partial M} &\displaystyle = \frac{\partial \epsilon}{\partial M} \frac{\partial}{\partial \epsilon} = \frac{2\epsilon}{M}\frac{\partial}{\partial \epsilon}\,,\\
\\
\displaystyle \frac{\partial}{\partial M} &\displaystyle = \frac{\partial \epsilon}{\partial M} \frac{\partial v}{\partial \epsilon} \frac{\partial}{\partial v} = -\frac{1-v^2}{Mv}\frac{\partial}{\partial v}\,.
\end{array}
\end{equation}
Therefore:
\begin{equation}
\begin{array}{rl}
\displaystyle \frac{\partial C_{2,g}^{(0)}}{\partial M}=&\displaystyle \frac{1}{M}T_R\Bigg\{2\epsilon\Big[2(-6-8\epsilon)I_2+4I_1+4J_2-4J_1\Big]\\
\\
&\displaystyle -\frac{1-v^2}{v}\Bigg[2(1-6\epsilon-4\epsilon^2)\frac{\partial I_2}{\partial v}-2(1-2\epsilon)\frac{\partial I_1}{\partial v}+\frac{\partial I_0}{\partial v}\\
\\
& \displaystyle -4(2-\epsilon)\frac{\partial J_2}{\partial v}+4(2-\epsilon)\frac{\partial J_1}{\partial v}-\frac{\partial J_0}{\partial v}\Bigg]\Bigg\}\,.
\end{array}
\end{equation}
To find the explicit expression, we just need to evaluate the
derivative of $I_q$ and $J_q$ starting from eqs. (\ref{eq:iq}) and
(\ref{eq:jq}) which is easily done:
\begin{equation}
\begin{array}{rcl}
\displaystyle \frac{\partial I_q}{\partial v} &=& \displaystyle\frac{2 z^q}{1-v^2}\,,\\
\\
\displaystyle \frac{\partial J_q}{\partial v} &=& \displaystyle z^q\,.
\end{array}
\end{equation}
In the end we get:
\begin{equation}\label{eq:dC2g0}
\begin{array}{rl}
\displaystyle \frac{\partial C_{2,g}^{(0)}}{\partial M}=&\displaystyle
                                                          \frac{1}{M}T_R\Bigg\{4\epsilon\left[(-6-8\epsilon)z^2+2z\right]\ln\left(\frac{1+v}{1-v}\right)+8\epsilon
                                                          z(z-1)v\\
\\
&\displaystyle -\frac{2}{v}\left[2(1-6\epsilon-4\epsilon^2)z^2-2(1-2\epsilon)z+1\right]\\
\\
& \displaystyle -\frac{1-v^2}{v}\left[-4(2-\epsilon)z^2+4(2-\epsilon)z-1\right]\Bigg\}\,.
\end{array}
\end{equation}

As is well known, the implementation of the FONLL scheme requires the
massless limit of the massive structure functions. In practice this
means that we need to compute the limit $M\rightarrow 0$ of the
massive coefficient functions retaining the logarithmic enhanced terms
and droping the power suppressed ones. To apply this recipe to
eq.~(\ref{eq:dC2g0}), we need to keep in mind that:
\begin{equation}
\epsilon \mathop{\longrightarrow}_{M\rightarrow 0} 0 \,,\quad v \mathop{\longrightarrow}_{M\rightarrow 0} 1\,,
\end{equation}
and that:
\begin{equation}
\ln\left(\frac{1+v}{1-v}\right) \mathop{\longrightarrow}_{M\rightarrow
  0} \ln\frac{Q^2(1-z)}{M^2z}\,,
\end{equation}
so that:
\begin{equation}\label{eq:dC2g00}
\displaystyle \frac{\partial C_{2,g}^{(0)}}{\partial M}\mathop{\longrightarrow}_{M\rightarrow 0}\displaystyle \frac{\partial C_{2,g}^{0,(0)}}{\partial M}=
                                                          -\frac{2}{M}T_R\left(2z^2-2z+1\right)\,.
\end{equation}

We now turn to consider $F_L$. In this case the the gluon coefficient
function takes the simpler form:
\begin{equation}
C_{L,g}^{(0)}\left(z,Q^2,M^2\right)= T_R\left[-8\epsilon I_2(\epsilon,z)-4J_2(\epsilon,z)+4J_1(\epsilon,z)\right]\,.
\end{equation}
Therefore, using eq. (\ref{eq:derivatives}), we immediately get:
\begin{equation}
\frac{\partial C_{L,g}^{(0)}}{\partial M} = \frac1{M}T_R\left[-16\epsilon
    z^2\ln\left(\frac{1+v}{1-v}\right) +\frac{8\epsilon z^2}{v}-\frac{1-v^2}{v}\left(-4z^2+4z\right)\right]\,.
\end{equation}
It is finally easy to realize that:
\begin{equation}
\frac{\partial C_{L,g}^{(0)}}{\partial
  M}\mathop{\longrightarrow}_{M\rightarrow 0} \frac{\partial C_{L,g}^{0,(0)}}{\partial M}=0\,.
\end{equation}
This concludes the treatment of the NC massive structure functions.

\subsubsection{Charged current}

In this section we consider the generic CC massive structure
function. The treatment is exactly the same of the NC structure
functions, with the only difference that in the CC case they start at
$\mathcal{O}(1)$ and they are presently known up to
$\mathcal{O}(a_s)$. This means that their perturbative expansion in
terms of the pole mass $M$ looks like this:
\begin{equation}
F_k(M) = F_k^{(0)}(M) + a_sF_k^{(1)}(M) + \mathcal{O}(a_s^2)\,,
\end{equation}
with $k=2,3,L$. Therefore, expanding $F^{(0)}$ and $F^{(1)}$ around $M=m$ and keeping only the terms up to $\mathcal{O}(a_s)$, one obtains:
\begin{equation}\label{eq:expCC}
F_k(m) = F_k^{(0)}(m) + a_s\left[F_k^{(1)}(m)+mh^{(1)}\frac{dF_k^{(0)}}{dM}\bigg|_{M=m}\right]\,.
\end{equation}

The leading-order contribution to the coefficient function can be
written as follows:
\begin{equation}
F^{(0)}_k(M) = b_k(M)s'(\xi(M))\,,
\end{equation}
where:
\begin{equation}\label{eq:definitions}
\xi = x\underbrace{\left(1+\frac{M^2}{Q^2}\right)}_{\frac1\lambda}=\frac{x}\lambda\quad\mbox{and}\quad
\left\{\begin{array}{l}
b_2 = \xi\\
b_3 = 1\\
b_L = (1-\lambda)\xi
\end{array}
\right.
\end{equation}
and where we have also defined:
\begin{equation}
s'\equiv 2|V_{cs}|^2s+2|V_{cd}|^2d\,.
\end{equation}
Therefore:
\begin{equation}\label{eq:derivCC}
\begin{array}{rcl}
\displaystyle mh^{(1)}\frac{dF^{(0)}_k}{dM}\bigg|_{M=m} &=&\displaystyle
  mh^{(1)}\frac{d\xi}{dM}\frac{dF^{(0)}_k}{d\xi}\bigg|_{M=m} \\
\\
&=&\displaystyle 
  2h^{(1)}(1-\lambda)\xi\left[\frac{db_k}{d\xi}s'(\xi)+b_k(\xi)\frac{ds'}{d\xi}\right]\bigg|_{M=m}\,,
\end{array}
\end{equation}
that can be conveniently rewritten as:
\begin{equation}
mh^{(1)}\frac{dF^{(0)}_k}{dM}\bigg|_{M=m} = 2h^{(1)}(1-\lambda)\left[\left(\frac{db_k}{d\xi}-\frac{b_k}{\xi}\right)+b_k(\xi)\frac{d}{d\xi}\right]\xi s'(\xi)\bigg|_{M=m}\,,
\end{equation}
so that, using eq.~(\ref{eq:definitions}), we have that:
\begin{equation}\label{eq:CCcorrections}
\begin{array}{rcl}
\displaystyle mh^{(1)}\frac{dF^{(0)}_2}{dM}\bigg|_{M=m} &=& \displaystyle
2h^{(1)}(1-\lambda)\xi\frac{d}{d\xi} \xi s'(\xi)\bigg|_{M=m}\,,\\
\\
\displaystyle mh^{(1)}\frac{dF^{(0)}_3}{dM}\bigg|_{M=m} &=& \displaystyle
2h^{(1)}(1-\lambda)\frac{1}{\xi}\left[ \xi\frac{d}{d\xi}-1\right]\xi
s'(\xi)\bigg|_{M=m}\,,\\
\\
\displaystyle mh^{(1)}\frac{dF^{(0)}_L}{dM}\bigg|_{M=m} &=& \displaystyle
2h^{(1)}(1-\lambda)^2\xi \frac{d}{d\xi}\xi s'(\xi)\bigg|_{M=m}\,.
\end{array}
\end{equation}

Finally, we notice that in the massless limit, where
$\lambda\rightarrow 1$, all expressions in
eq.~(\ref{eq:CCcorrections}) vanish, with the consequence that the CC
massive structure functions up to $\mathcal{O}(a_s)$ in terms of the
pole mass $M$ or the $\overline{\mbox{MS}}$ mass $m$ look exactly the
same.

As a last comment, the derivative of the PDF $s'$ that appears in
eq.~(\ref{eq:CCcorrections}) is implemented in {\tt APFEL} by means
the derivative of the Lagrange polynomials that are used to
interpolate PDFs.
